# Supplementary material for: Query Performance Prediction: From Ad-hoc to Conversational Search
Source: arXiv:2305.10923 source file (2023-05-18)
Supplement: Supplementary file 1 [file Appendix.tex]

\section*{Appendix}

A popular two-stage \ac{CS} pipeline~\citep{lin2021multi} can effectively solve this issue by
\begin{enumerate*}[label=(\roman*)]
\item first rewriting a conversational query into a self-contained query and then
\item reusing ad-hoc search systems fed with the query rewrite.
\end{enumerate*}

Inspired by the two-stage pipeline, we propose to model \ac{QPP} for \ac{CS} by feeding query rewrites to \ac{QPP} methods designed for ad-hoc search.

the RSVs are often less reliable for QPP because they are bounded within short intervals, diferent
 
Retrieval Status Values (RSVs).

Overall question: Do the lessons from QPP in a traditional search setting transfer to a conversational setting. 

This has two aspects: 
the absolute prediction scores of predictors (assuming we use metrics that are comparable), and
the relative prediction performance (if QPP-method A beats QPP-method B in a traditional setting, does A beat B in a conversational setting).

“does it generalize" questions: 
- do the relative performance QPP results known from traditional search still hold in a conversational setting?
-
are the relative QPP performance results in a conversational setting influenced by the choice of query rewriting?

We selected these three sets of queries to study the robustness of BERT-QPP w.r.t different query set sizes and relevance judgement schema. 

deep shallow pool in different datasets

models such as ours that are based on fine-tuning of contextual embedding show improved performance over large query sets

variations of BERTQPP approach show a stable performance on all three query sets

while NQA-QPP shows strong performance on MSMARCO dev set and TREC DL 2020 query set, it does not show a competitive performance on TREC DL 2019. 
A similar observation can be made for other strong baseline, namely UEF(NQC), which shows strong performance on TREC DL 2019 but not as competitive on the other two query sets, a

the score-based baselines perform poorly in predicting the performance of Conv-KNRM. This happens because the scale and distribution of the scores produced by neural models are different. 
Predicting the performance of BM25 is still easier for NQA-QPP, compared to the other retrieval models.

transforms the pointwise QPP objective into a listwise classification task
listwise outperform point wise

the number of documents the model consider
supervised bert QPP 1
unsupervised

Do the lessons from \ac{QPP} in ad-hoc search transfer to \ac{CS}?

the existing supervised approach for QPP, WS-NeurQPP, outperforms the unsupervised approaches (NQC, WIG and UEF),

Deep-QPP outperforms WS-NeurQPP, which confirms the hypothesis that explicitly learning the relative specificity of query pairs with an end-to end (strongly) supervised model is better able to generalize than a weakly supervised approach which learns an optimal combination
of statistical predictors

the aim of our reproducibility study is to 
In particular, the aim of our reproducibility study is to analyze investigate whether the findings of xx generalize along these dimensions

\begin{table*}[h]
\centering
\caption{
The results for predicting the performance of manual rewrites+BM25, in terms of reciprocal rank (RR). 
All models are fed with manual rewrites during training.
}
\label{6-1} 
\begin{tabular}{lccccccccc}
\toprule
  \multirow{2}{*}{\textbf{Methods}} & \multicolumn{3}{c}{OR-QuAC} & \multicolumn{3}{c}{CAsT-19} & \multicolumn{3}{c}{CAsT-20} \\
\cmidrule(lr){2-4} \cmidrule(lr){5-7}  \cmidrule(lr){8-10} 
 & Pearson   & Kendall  & Spearman   & Pearson   & Kendall  & Spearman     & Pearson   & Kendall  & Spearman \\
 \midrule
% T5 rewriting PPL & 0.307  & 0.227  & 0.315   & 0.174 & 0.167 & 0.226    & 0.058  & 0.017  & 0.024\\
%\midrule
%NQA-QPP  \\
%NeuralQPP             \\ 
BERT-QPP (manual rewrites during inference)   & 0.839   & 0.604   & 0.773        \\    
BERT-QPP (T5 rewrites during inference)   & 0.799  & 0.559   & 0.724       \\   
BERT-groupwise-QPP            \\  
qppBERT-PL   \\
%\midrule 
%xxx  \\ 
\bottomrule
\end{tabular}
%}
\end{table*}

\begin{table*}[t]
\centering
\caption{
The results for predicting the performance of T5 rewrites+BM25, in terms of reciprocal rank (RR). 
All models are fed with manual rewrites during training.
}
\label{6-1} 
\begin{tabular}{lccccccccc}
\toprule
  \multirow{2}{*}{\textbf{Methods}} & \multicolumn{3}{c}{OR-QuAC} & \multicolumn{3}{c}{CAsT-19} & \multicolumn{3}{c}{CAsT-20} \\
\cmidrule(lr){2-4} \cmidrule(lr){5-7}  \cmidrule(lr){8-10} 
 & Pearson   & Kendall  & Spearman   & Pearson   & Kendall  & Spearman     & Pearson   & Kendall  & Spearman \\
 \midrule
 %T5 rewriting PPL & 0.307  & 0.227  & 0.315   & 0.174 & 0.167 & 0.226    & 0.058  & 0.017  & 0.024\\
%\midrule
%NQA-QPP  \\
%NeuralQPP             \\ 
BERT-QPP (T5 rewrites during inference)   &  0.834  & 0.602 & 0.773        \\  
BERT-QPP (T5 rewrites during inference, trained on NDCG@3)   &  0.828  & 0.565 & 0.737        \\ 
BERT-QPP (manual rewrites during inference)   & 0.781   & 0.543  & 0.706      \\ 
BERT-groupwise-QPP            \\  
qppBERT-PL   \\
\midrule 
xxx  \\ 
\bottomrule
\end{tabular}
%}
\end{table*}

\begin{table*}[t]
\centering
\caption{
The results for predicting the performance of mannual rewrites+BM25, in terms of NDCG@3.
All models are fed with manual rewrites during training.
}
\label{6-1} 
\begin{tabular}{lccccccccc}
\toprule
  \multirow{2}{*}{\textbf{Methods}} & \multicolumn{3}{c}{OR-QuAC} & \multicolumn{3}{c}{CAsT-19} & \multicolumn{3}{c}{CAsT-20} \\
\cmidrule(lr){2-4} \cmidrule(lr){5-7}  \cmidrule(lr){8-10} 
 & Pearson   & Kendall  & Spearman   & Pearson   & Kendall  & Spearman     & Pearson   & Kendall  & Spearman \\
\midrule
%T5 rewriting PPL  & 0.259  & 0.212  & 0.278    & 0.205 & 0.174  & 0.246  &  0.061  & 0.048  & 0.064 \\
%\midrule
%NQA-QPP  \\
%NeuralQPP             \\ 
BERT-QPP (manual rewrites during inference)  & 0.792    &  0.562     & 0.705  \\
BERT-QPP (T5 rewrites during inference)   & 0.753   &  0.526   &  0.663        \\ 
BERT-groupwise-QPP            \\  
qppBERT-PL   \\
\midrule 
%xxx  \\ 
%\bottomrule
\end{tabular}
%}
\end{table*}

\begin{table*}[t]
\centering
\caption{
The results for predicting the performance of T5 rewrites+BM25, in terms of NDCG@3.
All models are fed with manual rewrites during training.
}
\label{6-1} 
\begin{tabular}{lccccccccc}
\toprule
  \multirow{2}{*}{\textbf{Methods}} & \multicolumn{3}{c}{OR-QuAC} & \multicolumn{3}{c}{CAsT-19} & \multicolumn{3}{c}{CAsT-20} \\
\cmidrule(lr){2-4} \cmidrule(lr){5-7}  \cmidrule(lr){8-10} 
 & Pearson   & Kendall  & Spearman   & Pearson   & Kendall  & Spearman     & Pearson   & Kendall  & Spearman \\
\midrule
%T5 rewriting PPL  & 0.259  & 0.212  & 0.278    & 0.205 & 0.174  & 0.246  &  0.061  & 0.048  & 0.064 \\
%\midrule
%NQA-QPP  \\
%NeuralQPP             \\ 
BERT-QPP (T5 rewrites during inference)   & 0.782   &  0.555  & 0.699         \\ 
BERT-QPP (T5 rewrites during inference, trained on RR)  & 0.785   & 0.565   & 0.710 \\
BERT-QPP (manual rewrites during inference)  & 0.730   & 0.507     & 0.642   \\
BERT-groupwise-QPP            \\  
qppBERT-PL   \\
%\midrule 
%xxx  \\ 
\bottomrule
\end{tabular}
%}
\end{table*}

\if0
\Acf{QPP} is a core task in information retrieval, that is to predict the performance of a retrieval model in response to a given query, when no relevance judgments are available.  

The evaluation of information retrieval systems outside the realm of the Cranfield paradigm~\citep{voorhees2001philosophy} (i.e., without access to relevance assessments) has been extensively explored in recent years~\citep{arabzadeh2021bert,chen2022groupwise,datta2022deep,datta2022relative,datta2022pointwise}.
This is because this evaluation paradigm can estimate the effectiveness of systems deployed in a real-life environment beyond the laboratory environment, and the estimated effectiveness is regarded as feedback to trigger the next actions of users or systems themselves.

\Acf{QPP} is an important specific task, that is to evaluate information retrieval systems without access to relevance assessments.
In other words, the QPP task aims to predict whether the retrieval method will be able to retrieve relevant documents for a certain query without having access to gold-standard relevance information for that query.
\ac{QPP} has been well-studied in ad-hoc retrieval~\citep{arabzadeh2021bert,chen2022groupwise,datta2022deep,datta2022relative,datta2022pointwise} and retrieval-based non-factoid question answering~\citep{hashemi2019performance}.
An effective \ac{QPP} method can play an important role in triggering query routing or query reformulation.

However, to the best of our knowledge, the evaluation of conversational retrieval systems~\citep{yu2021few} without access to relevance assessments has not been well-studied yet.
Although some existing studies try estimating the retrieval quality of a conversational retrieval system in a conversation scenario, they either directly utilise existing \ac{QPP} methods~\citep{lin2021multi} or only model single-turn conversation~\citep{arabzadeh2022unsupervised}.
Thus, they all ignore the multi-turn conversational nature/structure to facilitate the performance prediction in conversational retrieval.

In this paper, we introduce a new task, \acfi{CPP}, that is to automatically estimate the retrieval quality of a conversational retrieval system in a multi-turn conversation without access to relevance assessments.
\ac{CPP} can benefit conversational retrieval systems, especially mixed-initiative ones~\citep{aliannejadi2021building,aliannejadi2019asking,aliannejadi2020convai3}.
For instance, the system can take the initiative to ask a clarifying question to request more information from users when the estimated performance is poor.

We propose a xx model for \ac{CPP}. 

We regard state-of-the-art \ac{QPP} models as our baselines. 
Specifically, we adopt the state-of-the-art \ac{QPP} models to the \ac{CPP} task by utilising the widely-used T5 query writing method~\citep{lin2021multi} to rewrite a conversational context into a self-contained query.
Experiments on the two datasets~\citep{dalton2020cast,  
qu2020open} demonstrate that our proposed model can achieve state-of-the-art performance on the \ac{CPP} task.
\fi

%we cast \ac{QPP} for \ac{CS} as estimating the retrieval quality of an ad-hoc search system for the self-contained query rewrite of a conversational query.

%To check what is the performance of query performance prediction models in the conversational scenario? 
%Try to adapt query performance prediction models to the conversational scenario. 
%In the conversational scenario, to investigate in which cases query performance prediction models fail. 
%To find what kinds of features existing in the conversational scenario can be considered to improve conversation performance prediction and address the issues that query performance prediction models have. 
%To investigate to what extent the model considering these features improve the performance on conversation performance prediction compared to the adapted query performance prediction models. 
%To investigate to what extent the model considering these features improve the performance on the downstream system action prediction task compared to the adapted query 

%estimate how well the query has been satisfied by R 
%estimate the performance of a retrieved list of documents for a given input query
